# Supplementary material for: Robust Phantom-Assisted Framework for Multi-Person Localization and Vital Signs Monitoring Using MIMO FMCW Radar
Source: arXiv:2501.06755 source file (2025-01-12)
Supplement: Supplementary file 1 [file supp.pdf]

# Robust Phantom-Assisted Framework for Multi-Person Localization and Vital Signs Monitoring Using MIMO FMCW Radar - Supplementary Material

Yonathan Eder, *Graduate Student Member, IEEE*, Emma Zagoury, Shlomi Savariego, Moshe Namer, Oded Cohen, and Yonina C. Eldar, *Fellow, IEEE*

In this document, we provide the results of the single-person phantom trials c1 and the single-person human trials c2 to support and strengthen the conclusions of the main paper.

## A. Single-Person Phantom Trials

Fig. 1 presents the normalized localization maps within the designated ROI for trial #2 of class c1. We analyze the results of each method from left to right of each row: Although the *Angle-FFT* method exhibited a wide smearing effect, this did not hinder the detection of the subject's thorax in this single-person scenario, with only a minor angular error of 4 [°]. Both *MUSIC* and *SOD-MUSIC*, applied on each range-bin, incorrectly highlighted clutter in addition to the human target, resulting in inaccurate detection and positioning. While increasing the detection threshold may address this issue for single-person scenarios, it would significantly limit localization performance in multi-person cases. The *LCMV* map achieved an acceptable localization result, though it introduced an angular error of 7 [°]. The *cal-CIR* map successfully detected and positioned the subject with an angular error of only 3 [°], albeit with the presence of minor side lobes and smearing effects. Lastly, the proposed *RaLU-JSR* method generated a clean map with sharp detection lobe, achieving the smallest angular error of 2 [°]. Moreover, the narrow lobe width highlights the method's potential for accurate multi-target localization, as shown in Section V of the main paper.

Fig. 2 illustrates the NCVSM outcomes for this trial, generated by all 7 compared methods relative to the GT references, given the extracted  $\hat{v}_1$ . In this example, the estimated curves generally align with their respective reference curves across all methods, as expected given the relative simplicity of monitoring a single simulated subject via the custom phantom. Notably, while the refinement procedures (*PhaseReg+*, *FFT+*, and *OrthProj+*) improved the smoothness of the estimated curves and consequently enhanced performance, significant deviations from the reference curves were still observed at multiple time points for both HR and RR. Among the compared methods, the proposed E-VSDR exhibited the closest resemblance to the reference curves throughout the monitoring duration.

Fig. 3(a) shows the HR-AeCDF and RR-AeCDF of class c1. First, one sees that the E-VSDR outperforms all other

compared methods for every error threshold greater than 0.5 [bpm]. Specifically, it achieved an ASR2, ASR3, and ASR4 of 88.61%, 96.21%, and 97.33%, respectively, for HR estimation, and 99.38%, 100%, and 100%, respectively, for RR estimation. The values of the compared methods are given in Table I. Interestingly, the refinements applied to the competing methods yielded improvements primarily in RR estimation performance, yet they remained inferior to the E-VSDR. While the E-VSDR exhibited superior AeCDF performance, the relatively narrow performance gap in RR estimation can be attributed to the experimental setup. The single-person phantom trial generates distinct thoracic displacements directly in front of the radar antennas, enabling all methods to achieve reasonably accurate RR estimations.

Fig. 3(b) presents the HR-RMSE and RR-RMSE distributions for each NCVSM method across the 9 subjects of class c1, along with the corresponding average and median values. The proposed E-VSDR outperformed all other methods, achieving the lowest average and median RMSE for both HR and RR estimations, even when using the outlier-tolerant median metric. Specifically, the class ARMSE was as low as 1.18 and 0.49 for HR and RR estimation, respectively, with the values of the compared techniques given in Table I. Additionally, the E-VSDR obtained superior RMSE scores for most subjects, with only minor deviations observed for the remaining subjects. Observing the median RMSE, although refinements applied to *PhaseReg*, *FFT*, and *OrthProj* improved HR and RR estimation results, these enhancements remained insufficient to outperform the E-VSDR.

## B. Single-Person Human Trials

After drawing meaningful conclusions from the phantom trials, we proceeded with the human trials using similar parameters and configurations. The corresponding localization and NCVSM results for class c2 (single-person human trials) are presented below.

Fig. 4 below depicts the compared normalized localization maps for trial #7 of class c2, within the designated ROI. One can observe the following: 1. The *Angle-FFT* method incorrectly identified highly reflective clutter (at 0.9 and 1.02 [m]) located before the human target (at 1.37 [m]), with minimal power concentrated at the true position. 2. The

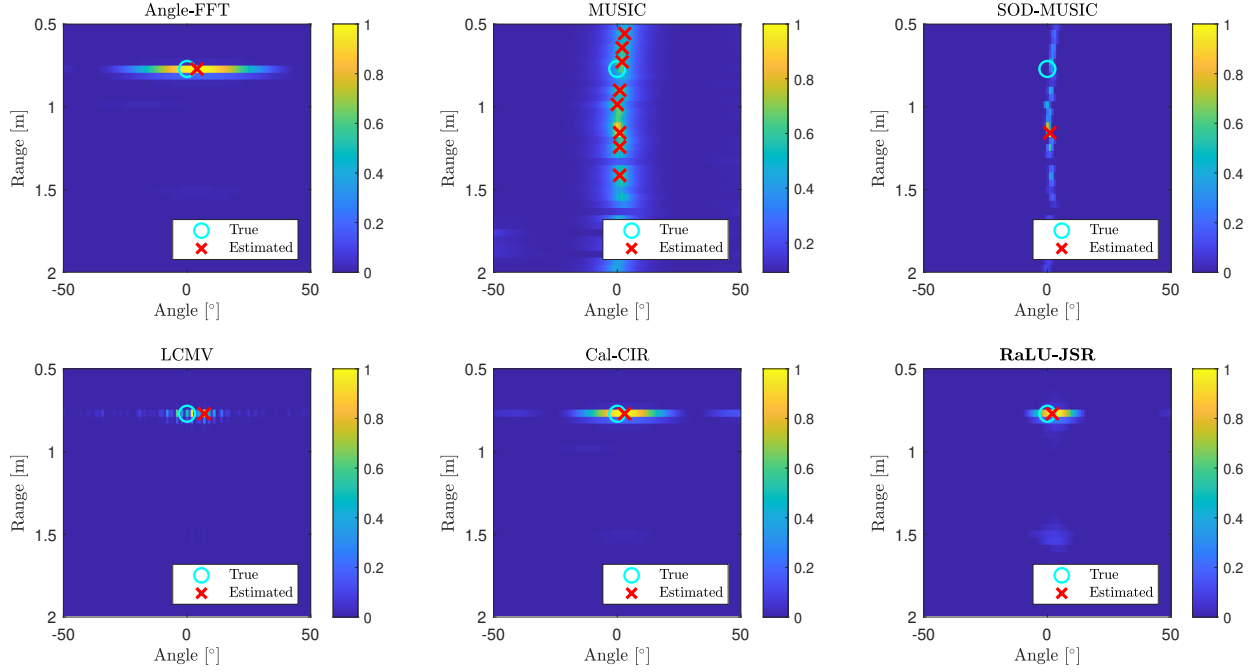

Fig. 1: Localization maps of single-person phantom trial - class c1, trial #2. The maps were produced by *Angle-FFT* [31]–[33], *MUSIC* [34], [35], *SOD-MUSIC* [36], *LCMV* [37], *cal-CIR* [38] and the proposed RaLU-JSR (Algorithm 1). The X and O signs denote the estimated and true locations of humans, respectively.

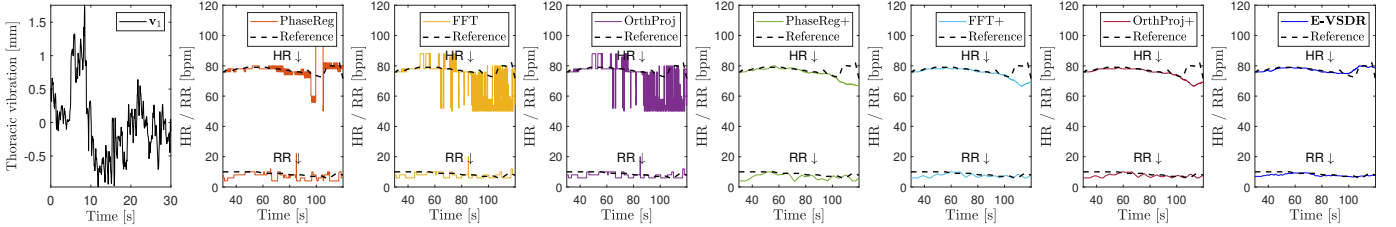

Fig. 2: NCVSM results for a single subject from trial #2 of class c1 (single-person phantom trials). **Columns:** Extracted thoracic vibration  $\hat{v}_1$  for a given  $T_{\text{int}}$ , *PhaseReg* [40], *FFT* [13]–[15], *OrthProj* [36], and their refined counterparts: *PhaseReg+*, *FFT+*, and *OrthProj+*. The rightmost plot presents the estimates by the proposed E-VSDR method, which achieved the closest alignment with the reference curves, surpassing competing approaches, even when they were enhanced by the proposed refinement procedure.

*MUSIC* algorithm detected returns near the true location but lacked the accuracy to precisely pinpoint the individual. 3. The enhanced *SOD-MUSIC* improved upon *MUSIC* by refining the output map and reducing clutter interference. However, it still failed to accurately position the detected subject. 4. The *LCMV* method focused on clutter at 0.9 [m], similar to *Angle-FFT*, leading to a misidentified location. 5. The *cal-CIR* map revealed reflections from both clutter (at 0.9 [m] and 1.02 [m]), and from the true subject location (at 1.37 [m]). However, its inability to effectively differentiate between clutter and human reflections resulted in incorrect selection of the clutter. 6. In contrast, the proposed RaLU-JSR precisely detected a single subject and accurately identified the position of its thorax, with an angular error of 4 [°], showcasing superior performance in both detection and positioning.

Fig. 5 illustrates the NCVSM results for this trial. Significant variability in HR estimates can be observed among the original compared methods (*PhaseReg*, *FFT*, and *OrthProj*), particularly in the later stages of the monitoring where a

rapid change in HR was observed. This variability deteriorated the ability to reliably monitor the HR, even with the refinements applied (*FFT+*, *OrthProj+*, and *PhaseReg+*). The E-VSDR not only produced an accurate RR estimates curve but also demonstrated exceptional robustness to challenging noise caused by interfering harmonics and rapid physiological state changes, effectively capturing the rapid HR fluctuations at the end of the monitoring period.

Fig. 6(a) presents the AeCDF results for HR and RR estimation across the 9 subjects in class c2. Consistent with the phantom trials, the E-VSDR outperformed all other methods for thresholds above 0.5 [bpm], achieving ASR2, ASR3, and ASR4 accuracies of 85.93%, 93.43%, and 96.91%, respectively, for HR estimation, and 97.00%, 100%, and 100%, respectively, for RR estimation. Detailed values for the compared methods are provided in Table I. While the refinements applied to the competing methods (*PhaseReg+*, *FFT+*, and *OrthProj+*) improved both HR and RR estimations compared to their unrefined counterparts, these enhancements were still

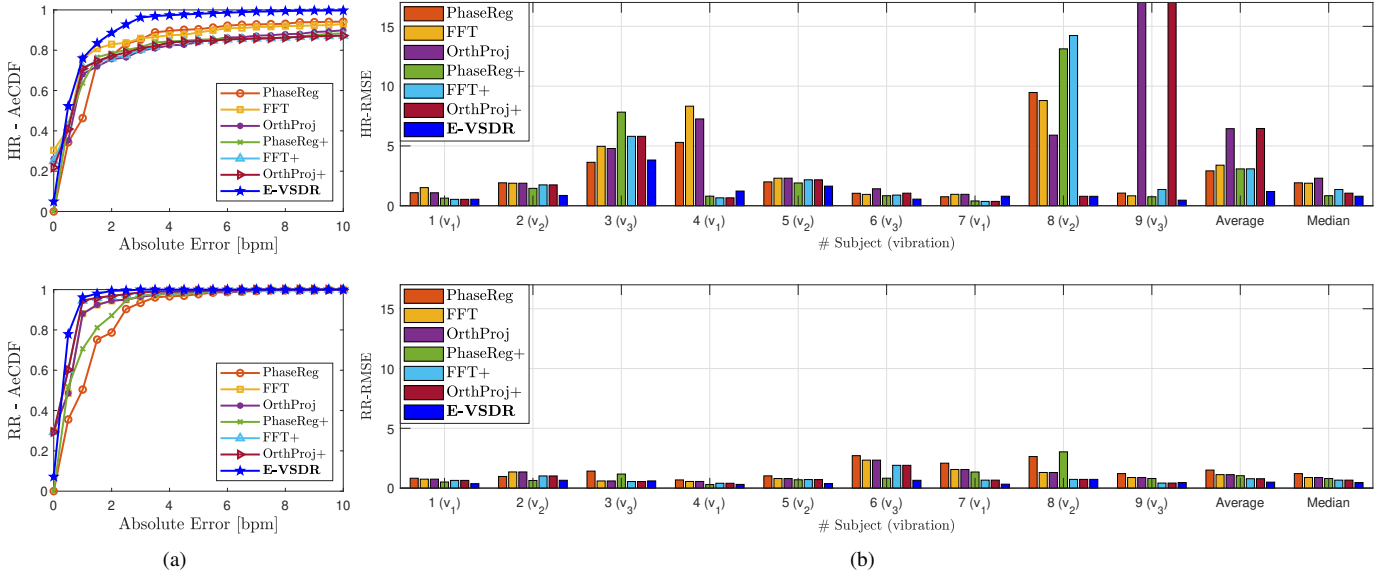

Fig. 3: NCVSM performance plots for multi-person phantom trials c3. (a) Average empirical CDFs for HR and RR estimations. (b) RMSE scores: subject-wise with class average and median. For both HR and RR estimations, the proposed E-VSDR outperformed the compared methods. In terms of AeCDF, it surpassed for every error above 0.5 [bpm], and in terms of RMSE, it achieved the lowest average and median values.

TABLE I: Average success rate [%] for 2 (ASR2), 3 (ASR3) and 4 (ASR4) [bpm] as well as average root-mean-squared-error (ARMSE) for HR and RR estimations by the compared NCVSM methods, for single-person classes c1 and c2.

| Class | Rate | Method           | ASR2         | ASR3         | ASR4         | ARMSE       |
|-------|------|------------------|--------------|--------------|--------------|-------------|
| c1    | HR   | <i>PhaseReg</i>  | 77.29        | 85.26        | 89.63        | 2.91        |
|       |      | <i>FFT</i>       | 82.99        | 85.91        | 87.48        | 3.39        |
|       |      | <i>OrthProj</i>  | 75.56        | 79.83        | 82.41        | 6.44        |
|       |      | <i>PhaseReg+</i> | 78.48        | 81.54        | 84.35        | 3.08        |
|       |      | <i>FFT+</i>      | 76.03        | 80.33        | 83.83        | 3.08        |
|       |      | <i>OrthProj+</i> | 77.20        | 81.01        | 83.83        | 6.45        |
|       |      | <b>E-VSDR</b>    | <b>88.61</b> | <b>96.21</b> | <b>97.33</b> | <b>1.18</b> |
|       | RR   | <i>PhaseReg</i>  | 78.69        | 93.44        | 96.64        | 1.50        |
|       |      | <i>FFT</i>       | 94.45        | 96.40        | 98.19        | 1.12        |
|       |      | <i>OrthProj</i>  | 94.45        | 96.40        | 98.19        | 1.12        |
|       |      | <i>PhaseReg+</i> | 87.11        | 96.99        | 97.83        | 1.03        |
|       |      | <i>FFT+</i>      | 96.85        | 98.63        | 99.08        | 0.78        |
|       |      | <i>OrthProj+</i> | 96.85        | 98.63        | 99.08        | 0.78        |
|       |      | <b>E-VSDR</b>    | <b>99.38</b> | <b>100</b>   | <b>100</b>   | <b>0.49</b> |
| c2    | HR   | <i>PhaseReg</i>  | 56.74        | 70.96        | 77.24        | 4.79        |
|       |      | <i>FFT</i>       | 60.42        | 67.18        | 70.54        | 6.20        |
|       |      | <i>OrthProj</i>  | 58.04        | 65.04        | 68.91        | 6.50        |
|       |      | <i>PhaseReg+</i> | 70.99        | 77.62        | 83.22        | 3.48        |
|       |      | <i>FFT+</i>      | 83.42        | 89.15        | 92.15        | 2.13        |
|       |      | <i>OrthProj+</i> | 80.04        | 87.36        | 90.81        | 2.27        |
|       |      | <b>E-VSDR</b>    | <b>85.93</b> | <b>93.43</b> | <b>96.91</b> | <b>1.45</b> |
|       | RR   | <i>PhaseReg</i>  | 81.54        | 89.63        | 94.08        | 2.21        |
|       |      | <i>FFT</i>       | 92.27        | 94.80        | 96.44        | 1.80        |
|       |      | <i>OrthProj</i>  | 92.27        | 94.80        | 96.44        | 1.80        |
|       |      | <i>PhaseReg+</i> | 91.18        | 96.59        | 98.10        | 1.00        |
|       |      | <i>FFT+</i>      | 96.37        | 98.41        | 100          | 0.74        |
|       |      | <i>OrthProj+</i> | 96.37        | 98.41        | 100          | 0.74        |
|       |      | <b>E-VSDR</b>    | <b>97.00</b> | <b>100</b>   | <b>100</b>   | <b>0.55</b> |

insufficient to surpass the performance of the E-VSDR, even in the single-person trials where the radar was directly aimed at the subject's thorax.

Finally, Fig. 6(b) illustrates the HR-RMSE and RR-RMSE

distributions for each NCVSM method across the 9 subjects in class c2. Similar to the phantom trials, the proposed E-VSDR achieved the lowest average and median RMSE values for both HR and RR estimations. Specifically, the class ARMSE was as low as 1.45 and 0.55 for HR and RR estimations, respectively, with the values for the compared methods presented in Table I. Furthermore, the refinements applied in *PhaseReg+*, *FFT+*, and *OrthProj+* resulted in improved performance for both HR and RR estimations, as observed for both the average and median metrics. However, even with these enhancements, these methods did not outperform the RMSE scores of the E-VSDR.

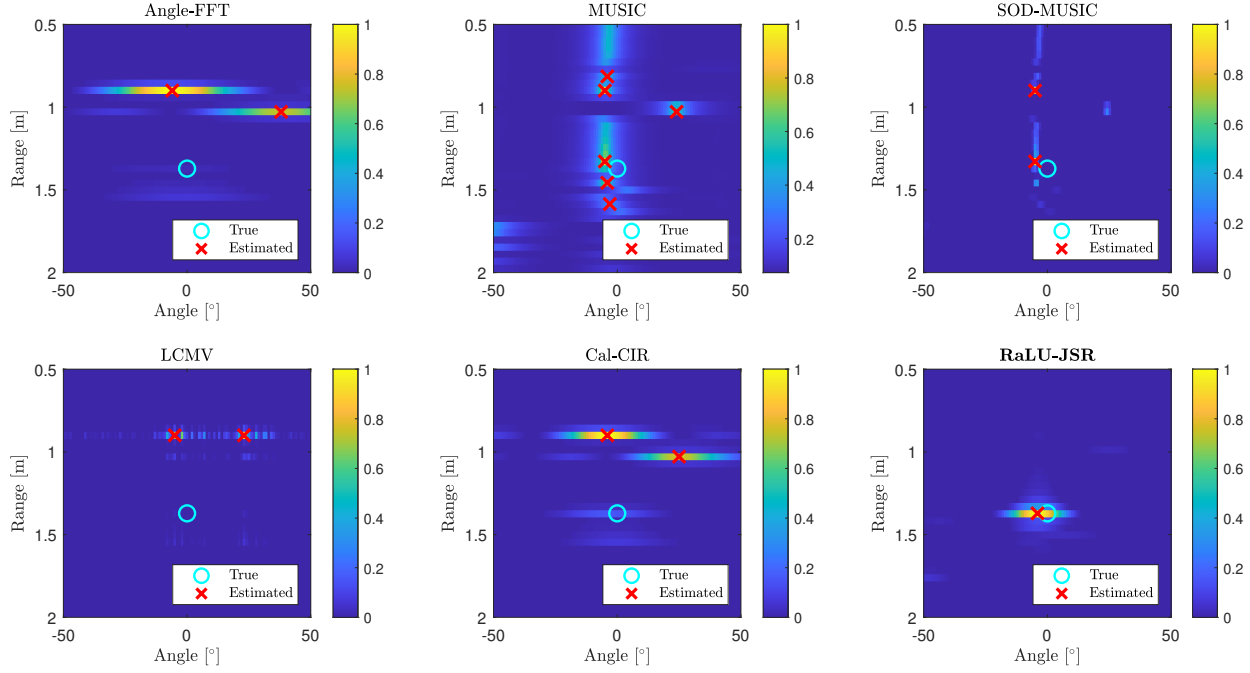

Fig. 4: Localization maps of single-person human trial - class c2, trial #7. The maps were produced by *Angle-FFT* [31]-[33], *MUSIC* [34], [35], *SOD-MUSIC* [36], *LCMV* [37], *cal-CIR* [38] and the proposed RaLU-JSR (Algorithm 1). The X and O signs denote the estimated and true locations of humans, respectively. Only the proposed RaLU-JSR properly detects and positions the subject in the specified scenario.

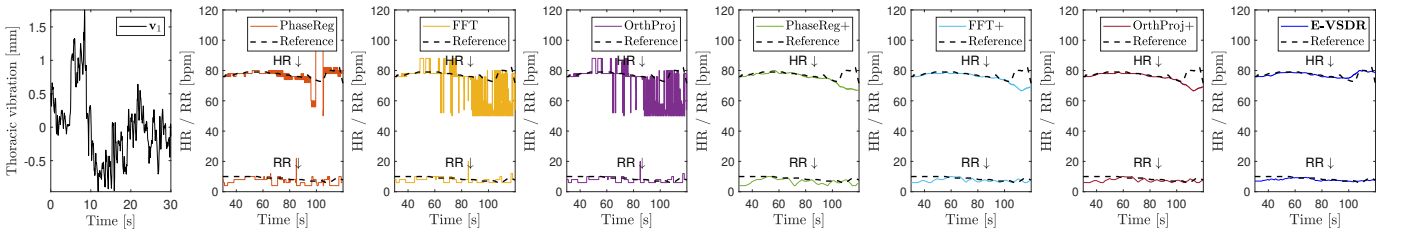

Fig. 5: NCVSM results for a single subject from trial #7 of class c2 (single-person human trials). **Columns:** Extracted thoracic vibration  $\hat{v}_1$  for a given  $T_{\text{int}}$ , *PhaseReg* [40], *FFT* [13]-[15], *OrthProj* [36], and their refined counterparts: *PhaseReg+*, *FFT+*, and *OrthProj+*. The rightmost plot presents the estimates by the proposed E-VSDR method, which achieved the closest alignment with the reference curves, surpassing competing approaches, even when they were enhanced by the proposed refinement procedure.

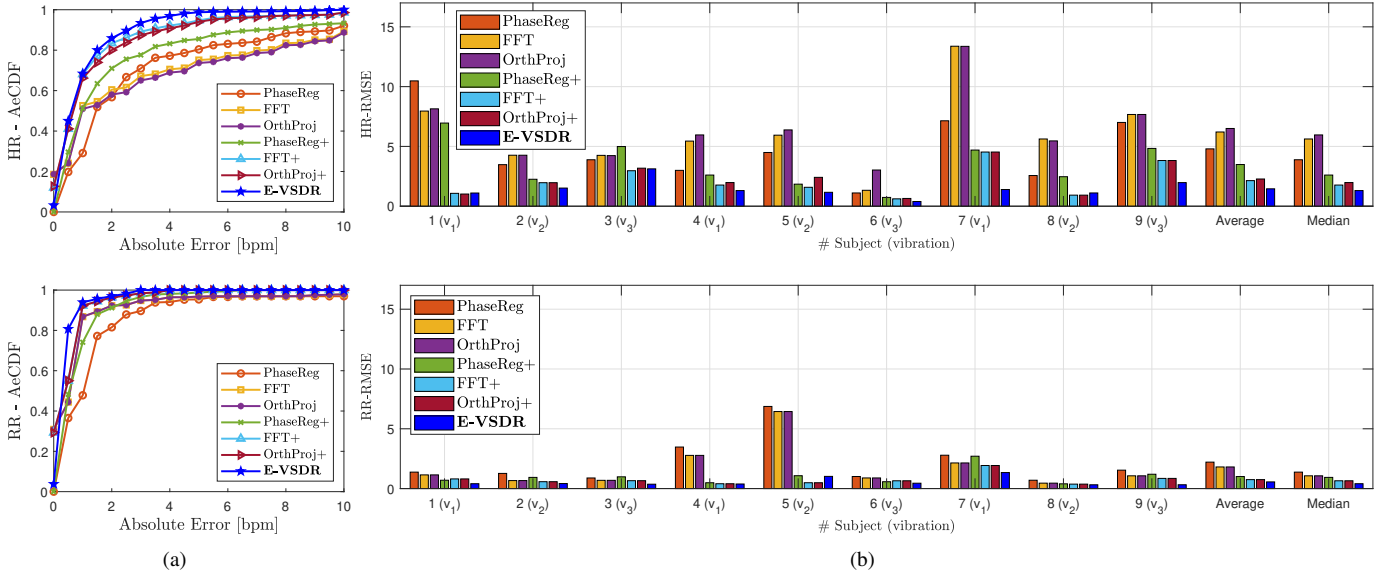

Fig. 6: NCVSM performance plots for single-person human trials c2. **(a)** Average empirical CDFs for HR and RR estimations. **(b)** RMSE scores: subject-wise with class average and median. For both HR and RR estimations, the proposed E-VSDR outperformed the compared methods. In terms of AeCDF, it surpassed for every error above 0.5 [bpm], and in terms of RMSE, it achieved the lowest average and median values.
